# Supplementary material for: Weak quantitative propagation of chaos via differential calculus on the space of measures
Source: arXiv:1901.02556 source file (2019-01-08)
Supplement: Supplementary file 1 [file appendix.tex]

%!TEX root = Particle_expansions_paper.tex
%\begin{subappendices}
%\renewcommand{\thesection}{A}%
%\arabic{section}

\appendix
\addcontentsline{toc}{section}{Appendices}
\section*{Appendices}
\section{Definition of classical solutions to PDEs in measure}

\begin{definition} \label{classical solution def} A function $\cV:[0,T]\times \cP_2(\R^d) \rightarrow \R$ is classical solution to \eqref{eq pde measure} if it satisfies the following conditions:
\begin{enumerate}[i)]
\item For all $t \in [0,T]$, $\cV(t,\cdot)$ is partially $C^2$.
\item Integrability condition: for every compact subset $\cK$ of $\cP_2(\R^d)$, the following holds:
\begin{align*}
\sup_{t \in [0,T], \mu \in \cK} \int \set{ |\partial_{\mu}\cV(t,\mu)(\upsilon)|^2 
+ 
|\partial_\upsilon \partial_{\mu}\cV(t,\mu)(\upsilon)|^2
} \, \mu(d\upsilon) < +\infty.
\end{align*}
\item For all $\mu \in \cP_{2}(\R^d)$, $\cV(\cdot,\mu)$ is  in $C^1([0,T])$.
%differentiable with continuous derivatives
\item The functions 
\begin{align*}
&[0,T]\times L^2(\R^d) \ni (t,\xi) \mapsto \partial_t \cV(t,\law[\xi]) \in \R
\\
&[0,T]\times L^2(\R^d) \ni (t,\xi) \mapsto \partial_\mu \cV(t,\law[\xi])(\xi) \in L^2(\R^d)
\\
&[0,T]\times L^2(\R^d) \ni (t,\xi) \mapsto \partial_\upsilon \partial_\mu \cV(t,\law[\xi])(\xi) \in L^2(\R^{d\times d})
\end{align*}
are continuous.
\end{enumerate}
\end{definition}
\section{Connection of linear functional derivatives and measure derivatives} \label{ lions functional} 

The bulk of this article focuses on the notion of derivatives in measure proposed by P. Lions (employed in many works on mean field games, such as \cite{buckdahn2017mean} and \cite{chassagneux2014probabilistic}),  which consists in working with a sufficiently large probability space $(\Omega, \cF, \bP)$ and looking at maps $U: \cP_2(\bR^d) \to \bR$
through their liftings to $L^2( \Omega, \cF, \bP; \bR^d)$ defined by 
$$ \widetilde{U}( X) = U(\law[X]), \quad \quad X \in L^2( \Omega, \cF, \bP; \bR^d).$$ 
We then represent its gradient as
$$ \nabla \widetilde{U} (X_0) = \pmu U( \law[X_0])(X_0),$$ 
for some function $\pmu U: \cP_2(\bR^d) \times \bR^d \to \bR^d$, if $\widetilde{U}$ is differentiable at $X_0$. Since $\pmu U$ can be viewed as a derivative in a vector field, it is natural to find a notion that serves as primitive functions of this differentiation process. 

A continuous function $\frac{\delta U}{\delta m}: \cP_2(\bR^d) \times \bR^d \to \bR$ is said to be the \emph{linear functional derivative} of $U: \cP_2(\bR^d) \to \bR$, if, for any $m, m' \in \cP_2(\bR^d)$,
$$ U(m')- U(m) = \int_0^1 \int_{\bR^d} \frac{\delta U}{\delta m}( (1-s)m + sm',y) \, (m'-m)(dy) \, ds. $$
Conventionally, it is normalised by
\begin{equation}
    \int_{\bR^d} \frac{\delta U}{\delta m}(m,y) \, m (dy) =0. \label{eq: normalisation first order linear functional deriatives} 
\end{equation}
Similarly,  a continuous function $\frac{\delta^2 U}{\delta m^2}: \cP_2(\bR^d) \times \bR^d \times \bR^d  \to \bR$ is said to be the \emph{second order linear functional derivative} of $U: \cP_2(\bR^d) \to \bR$ if, for any fixed $y \in \bR^d$ and any $m,m' \in \cP_2(\bR^d)$, 
$$ \frac{\delta U}{\delta m}(m',y) - \frac{\delta U}{\delta m} (m,y) = \int_0^1 \int_{\bR^d} \frac{\delta^2 U}{\delta m^2}((1-s)m +sm',y,y') \, (m'-m) (dy') \,ds.$$ 
As above, it is normalised by
\begin{equation}
    \int_{\bR^d} \frac{\delta^2 U}{\delta m^2}(m,y,y') \, m (dy') =0, \quad \quad \forall y \in \bR^d, \label{eq: normalisation second order linear functional deriatives 1} 
\end{equation}
and
\begin{equation}
    \int_{\bR^d} \frac{\delta^2 U}{\delta m^2}(m,y,y') \, m (dy) =0, \quad \quad \forall y' \in \bR^d. \label{eq: normalisation second order linear functional deriatives 2} 
\end{equation}
It is proven in \cite{carmona2017probabilistic} that if $\pmu U$ exists, then $\frac{\delta U}{\delta m}$ also exists and they are related by
\begin{equation}
    \pmu U(m,y) = D_y \frac{\delta U}{\delta m} (m,y). \label{eq: connection lions functional derivatives} 
\end{equation}
Similarly, if $\ptwomu U$ exists, then $\frac{\delta^2 U}{\delta m^2}$ also exists and they are related by
\begin{equation}
    \ptwomu U(m,y,y') = D^2_{y,y'} \frac{\delta^2 U}{\delta m^2} (m,y,y'). \label{eq: connection lions functional derivatives second order} 
\end{equation}
Similarly, we can derive similar properties for higher order linear functional derivatives. We mainly work with functions in  class $\cM_k$ in this article, but nonetheless require conditions of regularity for linear functional derivatives in Propositions \ref{pr expansion initial condition} and \ref{ proposition second order expansion}. The following proposition gives a link between regularity of Lions derivatives and regularity of linear functional derivatives.  
\begin{proposition} \label{theorem lions linear functional} 
Suppose that $U \in \cM_k ( \cP_2 (\bR^d))$.  Then
\begin{equation} \bigg| \frac{\delta^k U}{\delta m^k} (m,y_1, \ldots, y_k) \bigg| \leq C \bigg( |y_1|^k + \ldots +  |y_k|^k + \int_{\bR^d} |x|^k \, m(dx) \bigg). \label{eq: higher order lions linear functional} \end{equation} 
\begin{comment}
and
\begin{eqnarray}
&& \bigg| \frac{\delta^2 U}{\delta m^2} (m,y_1, y_2) - \frac{\delta^2 U}{\delta m^2} (m',y_1, y_2) \bigg| \nonumber \\
& \leq &  W_2 (m,m') \bigg[ \Big( 9 \| \ptwomu U\|_{\text{Lip}} + 2 \|\ptwomu U\|_{\infty}  \Big) \bigg( 2 + |y_1|^2 + |y_2|^2 + \int_{\bR} |x|^2 \, m(dx) + \int_{\bR} |x|^2 \, m'(dx) \bigg) \bigg].   \nonumber \\
&& \label{eq: second order lions linear functional 2} 
\end{eqnarray}
\end{comment}
\end{proposition}
\begin{proof}
For simplicity of notations, the proof is presented in dimension one. We present a sketch of the proof for $k=1$ and $k=2$.  By \eqref{eq: connection lions functional derivatives} and the fundamental theorem of calculus,  
$$ \frac{\delta U}{\delta m} (m,y) - \frac{\delta U}{\delta m} (m,y') = \int_{y'}^y \pmu U(m,s) \, ds. $$ 
The property of normalisation \eqref{eq: normalisation second order linear functional deriatives 1}  gives
$$\frac{\delta U}{\delta m} (m,y)  = \int_{\bR} \int_{y'}^y \pmu U(m,s) \, ds \, m(dy').  $$ 
By the supremum bound on $\pmu U$, we have
\begin{equation}  \bigg| \frac{\delta U}{\delta m} (m,y) \bigg|  \leq \int_{\bR} \| \pmu U \|_{\infty} |y-y'| m(dy') \leq \| \pmu U \|_{\infty}  \bigg( |y| + \int_{\bR} |x| \, m(dx) \bigg).  \nonumber 
\end{equation}
%\label{eq: first order linear functional derivation extended}} 
The argument is similar for the statement pertaining to second order derivatives. 
By \eqref{eq: connection lions functional derivatives second order} and the fundamental theorem of calculus,
\begin{eqnarray}
&& \frac{\delta^2 U}{\delta m^2} (m,y_1, y_2) - \frac{\delta^2 U}{\delta m^2} (m,y_1, y'_2) \nonumber \\
& = & \int_{y'_2}^{y_2} D_{x_2} \bigg[ \frac{\delta^2 U}{\delta m^2} (m,y_1,u) \bigg]\, du \nonumber \\ 
& = & \int_{y'_2}^{y_2} D_{x_2} \bigg[ \frac{\delta^2 U}{\delta m^2} (m,y_1,u) \bigg]\, du - \int_{y'_2}^{y_2} D_{x_2} \bigg[ \frac{\delta^2 U}{\delta m^2} (m,y'_1,u) \bigg]\, du + \int_{y'_2}^{y_2} D_{x_2} \bigg[ \frac{\delta^2 U}{\delta m^2} (m,y'_1,u) \bigg]\, du \nonumber \\
& = & \int_{y'_2}^{y_2} \int_{y'_1}^{y_1} \ptwomu U(m,s,u) \, ds \,du + \int_{y'_2}^{y_2} D_{x_2} \bigg[ \frac{\delta^2 U}{\delta m^2} (m,y'_1,u) \bigg]\, du, \nonumber 
\end{eqnarray}
which implies that
$$ \frac{\delta^2 U}{\delta m^2} (m,y_1, y_2) = \int_{y'_2}^{y_2} \int_{y'_1}^{y_1} \ptwomu U(m,s,u) \, ds \,du + \int_{y'_2}^{y_2} D_{x_2} \bigg[ \frac{\delta^2 U}{\delta m^2} (m,y'_1,u) \bigg]\, du + \frac{\delta^2 U}{\delta m^2} (m,y_1, y'_2). $$ 
By \eqref{eq: normalisation second order linear functional deriatives 1} and \eqref{eq: normalisation second order linear functional deriatives 2}, we have
\begin{equation} \frac{\delta^2 U}{\delta m^2} (m,y_1, y_2) = \int_{\bR} \int_{\bR} \int_{y'_2}^{y_2} \int_{y'_1}^{y_1} \ptwomu U(m,s,u) \, ds \,du \, m(dy'_1) \, m(dy'_2). \nonumber  \end{equation}
% \label{eq: second order functional derivatives normalised form} 
Therefore,
\begin{eqnarray}
\bigg| \frac{\delta^2 U}{\delta m^2} (m,y_1, y_2) \bigg| & \leq & \int_{\bR} \int_{\bR} \| \ptwomu U\|_{\infty} |y_1 - y'_1| |y_2- y'_2| \, m(dy'_1) \, m(dy'_2) \nonumber \\
& \leq & \| \ptwomu U\|_{\infty} \bigg( |y_1| + \int_{\bR} |x| \, m(dx) \bigg) \bigg( |y_2| + \int_{\bR} |x| \, m(dx) \bigg) \nonumber \\
& \leq & \| \ptwomu U\|_{\infty} \bigg( |y_1| + |y_2| + \int_{\bR} |x| \, m(dx) \bigg)^2 \nonumber \\
& \leq & 9  \| \ptwomu U\|_{\infty} \bigg( |y_1|^2 + |y_2|^2 + \int_{\bR} |x|^2 \, m(dx) \bigg). \nonumber 
\end{eqnarray}
\end{proof}
%\end{subappendices}
\newpage
